# Supplementary material for: Isogeometric Analysis of Acoustic Scattering using Infinite Elements
Source: arXiv:2204.09505 source file (2022-04-20)
Supplement: Supplementary file 1 [file analyticSolutionsAppendix.tex]

\section{Analytic solutions}
\label{Sec2:AnalyticSolutions}
For scattering on spheres and layers of spherical shells, we can obtain analytic solutions. Due to spherical symmetry, we can generalize this solution for arbitrary incident plane waves (characterised by $\vec{k}=\vec{k}(\alpha_{\mathrm{s}},\beta_{\mathrm{s}})$) by a simple orthogonal transformation, so it suffices to consider the case with $\vec{k}=[0, 0, k]^\transpose$.

\subsection{Plane wave scattered by a rigid sphere}
Let the plane wave\footnote{We here use the spherical coordinate system where $r\in[0,\infty)$ is the radius, $\vartheta\in[0,\PI]$ is the polar angle and $\varphi\in[0,2\PI)$ is the asimuth angle satisfying the relations
\begin{equation*}
	x = r\sin\vartheta\cos\varphi,\quad y = r\sin\vartheta\sin\varphi,\quad z = r\cos\vartheta.
\end{equation*}
} (with $\vec{k}=[0, 0, k]^\transpose$)
\begin{equation*}
	p_{\textrm{inc}}(r,\vartheta) = P_{\mathrm{inc}}\euler^{\imag kz} = P_{\mathrm{inc}}\euler^{\imag kr\cos\vartheta}
\end{equation*}
be scattered on a sphere with radius $R=0.5$. The resulting scattered wave is then\footnote{Here, $P_n(x)$ denotes the $n^{\mathrm{th}}$ Legendre polynomial and $j_n(x)$ denotes the $n^{\mathrm{th}}$ spherical Bessel function of first kind, and $h_n(x)$ denotes the $n^{\mathrm{th}}$ spherical Hankel function of the first kind.} (rigid scattering)
\begin{equation}\label{Eq2:rigidScattering_p}
	p_{\mathrm{rs}} (r,\vartheta) = -P_{\mathrm{inc}}\sum_{n=0}^\infty \imag^n (2n+1) P_n(\cos\vartheta)\frac{j_n'(kR)}{h_n'(kR)} h_n(kr).
\end{equation}
When computing the $H^1$-norm of the error we will also need the corresponding gradient, which in spherical coordinates is given by
\begin{align*}
	\nabla p_{\mathrm{rs}} (r,\vartheta) &= \pderiv{p_{\mathrm{rs}}}{r}\vec{e}_{\mathrm{r}} + \frac{1}{r}\pderiv{p_{\mathrm{rs}}}{\vartheta}\vec{e}_{\upvartheta} + \frac{1}{r\sin\vartheta}\pderiv{p_{\mathrm{rs}}}{\varphi}\vec{e}_{\upvarphi}\\
	&= -P_{\mathrm{inc}}\sum_{n=0}^\infty \imag^n (2n+1) \frac{j_n'(kR)}{h_n'(kR)} \left(P_n(\cos\vartheta)kh_n'(kr)\vec{e}_{\mathrm{r}} - \frac{\sin\vartheta}{r}P_n'(\cos\vartheta)h_n(kr)\vec{e}_{\upvartheta}\right)
\end{align*}
where the involved unit vectors in spherical coordinates are related to the Cartesian coordinates by
\begin{align*}
	\vec{e}_{\mathrm{r}} &= \sin\vartheta\cos\varphi\vec{e}_{\mathrm{x}} + \sin\vartheta\vec{e}_{\mathrm{y}} + \cos\vartheta\vec{e}_{\mathrm{z}}\\
	\vec{e}_{\upvartheta} &= \cos\vartheta\cos\varphi\vec{e}_{\mathrm{x}} + \cos\vartheta\sin\varphi\vec{e}_{\mathrm{y}} - \sin\vartheta\vec{e}_{\mathrm{z}}.
\end{align*}
For details of this solution see Ihlenburg~\cite[p. 28]{Ihlenburg1998fea}.

\subsection{Plane wave scattered by an elastic spherical shell}
In~\cite[pp. 12-20]{Chang1994voa} the exact 3D elasticity solution for the spherical shell is presented. We shall repeat the final formulas needed for the scattered pressure.
Let the plane wave
\begin{equation*}
	p_{\textrm{inc}}(r,\vartheta) = P_{\mathrm{inc}}\euler^{\imag kz} = P_{\mathrm{inc}}\euler^{\imag kr\cos\vartheta}
\end{equation*}
be scattered on a elastic spherical shell with inner radius $R_1$ and outer radius $R_0$. The scattered pressure is then\footnote{Here, $P_n(x)$ denotes the $n^{\mathrm{th}}$ Legendre polynomial, $j_n(x)$ and $y_n(x)$ denotes the $n^{\mathrm{th}}$ spherical Bessel function of first and second kind, respectively, and $h_n(x)$ denotes the $n^{\mathrm{th}}$ spherical Hankel function of the first kind.}  (elastic scattering)
\begin{equation}\label{Eq2:exact3DscatteringSphericalShellSol}
	p_{\mathrm{es}}(r,\vartheta) = p_{\mathrm{rs}}(r,\vartheta) + \frac{P_{\mathrm{inc}}\rho_{\mathrm{f}} c_{\mathrm{f}}}{(kR_0)^2}\sum_{n=0}^\infty \frac{\imag^n(2n+1)P_n(\cos\vartheta)h_n(kr)}{[h_n'(kR_0)]^2(Z_n+z_n)}
\end{equation}
where $p_{\mathrm{rs}}$ is defined in \Cref{Eq2:rigidScattering_p}, and $z_n$ (\textit{specific acoustic impedance}) and $Z_n$ (\textit{mechanical impedance}) are defined by
\begin{equation*}
	z_n = \imag\rho_{\mathrm{f}} c_{\mathrm{f}}\frac{h_n(kR_0)}{h_n'(kR_0)}
\end{equation*}
and
\begin{equation*}
	Z_n =\frac{R_0}{-\imag\omega\left[C_n^{(1)} D_{1,n}^{(1)}(b_1 R_0) + C_n^{(2)} D_{2,n}^{(1)}(b_2 R_0) + C_n^{(3)} D_{1,n}^{(2)}(b_1 R_0) + C_n^{(4)} D_{2,n}^{(2)}(b_2 R_0)\right]},
\end{equation*}
where 
\begin{equation*}
	D_{1,n}^{(i)}(x) = nA_n^{(i)}(x)-xA_{n+1}^{(i)}(x),\quad\text{and}\quad	D_{2,n}^{(i)}(x) = n(n+1)A_n^{(i)}(x),
\end{equation*}
and the coefficients $C_n^{(1)}$, $C_n^{(2)}$, $C_n^{(3)}$ and $C_n^{(4)}$ are given by
\begin{equation*}
	C_0^{(1)} = \frac{\frac{R_0^2}{2\mu}B_{1,n}^{(2)}(b_1 R_1)}{\nabla^2_0},\quad C_0^{(2)}=0,\quad	C_0^{(3)} = -\frac{\frac{R_0^2}{2\mu}B_{1,n}^{(1)}(b_1 R_1)}{\nabla^2_0},\quad C_0^{(4)}=0,
\end{equation*}
for $n=0$ where
\begin{equation*}
	\nabla^2_0=\begin{vmatrix}
		B_{1,n}^{(1)}(b_1 R_0) & B_{1,n}^{(2)}(b_1 R_0)\\
		B_{1,n}^{(1)}(b_1 R_1) & B_{1,n}^{(2)}(b_1 R_1)
	\end{vmatrix},
\end{equation*}
and by
\begin{equation*}
	C_n^{(1)} = \frac{\nabla^2_{1,n}}{\nabla^2_n},\quad C_n^{(2)} = \frac{\nabla^2_{2,n}}{\nabla^2_n},\quad C_n^{(3)} = \frac{\nabla^2_{3,n}}{\nabla^2_n},\quad C_n^{(4)} = \frac{\nabla^2_{4,n}}{\nabla^2_n},
\end{equation*}
for $n>0$ where the following notations has been used
\begin{equation*}
	\nabla^2_n = \begin{vmatrix}
		B_{1,n}^{(1)}(b_1 R_0) & B_{2,n}^{(1)}(b_2 R_0) & B_{1,n}^{(2)}(b_1 R_0) & B_{2,n}^{(2)}(b_2 R_0)\\
		B_{1,n}^{(1)}(b_1 R_1) & B_{2,n}^{(1)}(b_2 R_1) & B_{1,n}^{(2)}(b_1 R_1) & B_{2,n}^{(2)}(b_2 R_1)\\
		B_{3,n}^{(1)}(b_1 R_0) & B_{4,n}^{(1)}(b_2 R_0) & B_{3,n}^{(2)}(b_1 R_0) & B_{4,n}^{(2)}(b_2 R_0)\\
		B_{3,n}^{(1)}(b_1 R_1) & B_{4,n}^{(1)}(b_2 R_1) & B_{3,n}^{(2)}(b_1 R_1) & B_{4,n}^{(2)}(b_2 R_1)
	\end{vmatrix},
\end{equation*}
\begin{equation*}
	\nabla^2_{1,n} = \frac{R_0^2}{2\mu}\begin{vmatrix}
		B_{2,n}^{(1)}(b_2 R_1) & B_{1,n}^{(2)}(b_1 R_1) & B_{2,n}^{(2)}(b_2 R_1)\\
		B_{4,n}^{(1)}(b_2 R_0) & B_{3,n}^{(2)}(b_1 R_0) & B_{4,n}^{(2)}(b_2 R_0)\\
		B_{4,n}^{(1)}(b_2 R_1) & B_{3,n}^{(2)}(b_1 R_1) & B_{4,n}^{(2)}(b_2 R_1)
	\end{vmatrix},
\end{equation*}
\begin{equation*}
	\nabla^2_{2,n} = -\frac{R_0^2}{2\mu}\begin{vmatrix}
		B_{1,n}^{(1)}(b_1 R_1) & B_{1,n}^{(2)}(b_1 R_1) & B_{2,n}^{(2)}(b_2 R_1)\\
		B_{3,n}^{(1)}(b_1 R_0) & B_{3,n}^{(2)}(b_1 R_0) & B_{4,n}^{(2)}(b_2 R_0)\\
		B_{3,n}^{(1)}(b_1 R_1) & B_{3,n}^{(2)}(b_1 R_1) & B_{4,n}^{(2)}(b_2 R_1)
	\end{vmatrix},
\end{equation*}
\begin{equation*}
	\nabla^2_{3,n} = \frac{R_0^2}{2\mu}\begin{vmatrix}
		B_{1,n}^{(1)}(b_1 R_1) & B_{2,n}^{(1)}(b_2 R_1) & B_{2,n}^{(2)}(b_2 R_1)\\
		B_{3,n}^{(1)}(b_1 R_0) & B_{4,n}^{(1)}(b_2 R_0) & B_{4,n}^{(2)}(b_2 R_0)\\
		B_{3,n}^{(1)}(b_1 R_1) & B_{4,n}^{(1)}(b_2 R_1) & B_{4,n}^{(2)}(b_2 R_1)
	\end{vmatrix},
\end{equation*}
\begin{equation*}
	\nabla^2_{4,n} = -\frac{R_0^2}{2\mu}\begin{vmatrix}
		B_{1,n}^{(1)}(b_1 R_1) & B_{2,n}^{(1)}(b_2 R_1) & B_{1,n}^{(2)}(b_1 R_1)\\
		B_{3,n}^{(1)}(b_1 R_0) & B_{4,n}^{(1)}(b_2 R_0) & B_{3,n}^{(2)}(b_1 R_0)\\
		B_{3,n}^{(1)}(b_1 R_1) & B_{4,n}^{(1)}(b_2 R_1) & B_{3,n}^{(2)}(b_1 R_1)
	\end{vmatrix},
\end{equation*}
\begin{align*}
	B_{1,n}^{(i)}(x) &= \left[n^2-n-\frac{1}{2}\left(\frac{b_2}{b_1}\right)^2 x^2\right] A_n^{(i)}(x) + 2xA_{n+1}^{(i)}(x),\\
	B_{2,n}^{(i)}(x) &= n(n+1)\left[(n-1)A_n^{(i)}(x) - xA_{n+1}^{(i)}(x)\right],\\
	B_{3,n}^{(i)}(x) &= (n-1) A_n^{(i)}(x) - xA_{n+1}^{(i)}(x),\\
	B_{4,n}^{(i)}(x) &= \left(n^2-1-\frac{1}{2}x^2\right) A_n^{(i)}(x) + xA_{n+1}^{(i)}(x),
\end{align*}
%\begin{align*}
%	B_9^{(i)}(x) &= \left[-n^2-\frac{1}{2}\left(\frac{b_2}{b_1}\right)^2 x^2+x^2\right] A_n^{(i)}(x) - xA_{n+1}^{(i)}(x)\\
%	B_7^{(i)}(x) &= -(n^2+n)\left[n A_n^{(i)}(x) - xA_{n+1}^{(i)}(x)\right] \\
%	B_5^{(i)}(x) &= \left[n-\frac{1}{2}x^2+\left(\frac{b_1}{b_2}\right)^2 x^2\right] A_n^{(i)}\left(\frac{b_1}{b_2}x\right) - \frac{b_1}{b_2}x A_{n+1}^{(i)}\left(\frac{b_1}{b_2}x\right)\\
%	B_6^{(i)}(x) &= n(n+1)A_n^{(i)}(x)\\
%\end{align*}
\begin{equation*}
	A_{n}^{(1)}(x) = j_n(x),\qquad A_{n}^{(2)}(x) = y_n(x),
\end{equation*}
\begin{equation*}
	b_1=\frac{\omega}{c_1},\quad b_2=\frac{\omega}{c_2},\quad c_1 = \sqrt{\frac{\lambda+2\mu}{\rho_s}},\quad c_2 = \sqrt{\frac{\mu}{\rho_s}}.
\end{equation*}
Here, the parameters $c_1$ and $c_2$ are called the longitudinal wave velocity and shear wave velocity, respectively. Moreover, $\lambda$ and $\mu$ are the Lam{\'e} parameters which can be defined by the Young's modulus, $E$, and Poisson's ratio, $\nu$, as
\begin{equation*}
	\lambda = \frac{\nu E}{(1+\nu)(1-2\nu)}\quad\text{and}\quad \mu = \frac{E}{2(1+\nu)}.
\end{equation*}
